# Supplementary material for: Semiconducting van der Waals Interfaces as Artificial Semiconductors
Source: arXiv:1807.08282 ancillary file (2018-07-22)
Supplement: Supplementary file 1 [file SI_vdW_interfaces_Ponomarev_resub2.pdf]

# Supporting information

# Semiconducting van der Waals Interfaces as Artificial Semiconductors

Evgeniy Ponomarev,[†] Nicolas Ubrig,[†] Ignacio Gutiérrez-Lezama,[†] Helmuth Berger,[‡] and Alberto F. Morpurgo[*,†]

†*DQMP and GAP, Université de Genève, 24 quai Ernest Ansermet, CH-1211, Geneva, Switzerland*

‡*Institut de Physique de la Matière Complexe, EPFL, CH-1015 Lausanne, Switzerland*

E-mail: Alberto.Morpurgo@unige.ch

## S1 Methods

*Device Fabrication.* The fabrication of the devices used to perform the measurements discussed in the main text relies on a combination of conventional nano-fabrication techniques and of techniques that are commonly employed to manipulate atomically thin crystals, *i.e.*, 2D materials. Monolayers of $MoS_2$, $MoSe_2$, and $WSe_2$ are obtained by mechanical exfoliation of bulk crystals; the crystals of $MoS_2$ and $MoSe_2$ were purchased from different companies (2D semiconductors and HQ graphene) and the $WSe_2$ crystals were grown in-house by means of a chemical vapor transport technique. The exfoliated crystals were transferred onto $Si/SiO_2$ substrate and the monolayers were identified by looking at their optical contrast under an optical microscope, and by doing photoluminescence spectroscopy measurements. For the realization of the devices

discussed in the main text we took care to select large area monolayers of the different materials, so that once transferred to form the interfaces, a sufficiently large part of the individual monolayers could also be contacted and used in a field-effect transistor configuration.

To realize transistor devices once the two monolayers are properly positioned (see Figure 1 of the main text), a conventional process based on electron beam lithography, electron-beam evaporation and lift-off is used to attach electrical contacts to the interface and the two monolayers (the contacts consist of Pt/Au evaporated films, with Pt in contact with the monolayers), as well as a large gate electrode and an additional so-called reference electrode (to measure the voltage drop $V_{ref}$ between the liquid and the device). Finally the ionic liquid is applied on top of the structure and the device is mounted in the vacuum chamber used to perform electrical measurements ($p \simeq 10^{-6}$ mbar) as rapidly as possible to minimize exposure to air (the devices are left under vacuum at least overnight prior to the application of any gate bias to ensure that humidity or oxygen possibly present are pumped out of the system). The ionic liquid that was used in all experiments discussed here is 1-butyl-1-methylpyrrolidiniumtris(pentafluoroethyl) trifluorophosphate [P14][FAP].

*Transport and optoelectronic measurements.* Transport experiments – *i.e.,* the measurements of the output and transfer transistor curves discussed in the main text – were done in a voltage-bias configuration using low-noise home-made electronics to source voltage and measure current. Photoluminescence measurements were performed in a backscattering geometry, by using an optical microscope to illuminate the device with the incoming laser beam and to collect the resulting emitted light. The light collected from the sample was sent to a Czerny-Turner monochromator and detected with a Si CCD array (Andor). The laser excitation wavelength was set to 514.5 nm, and the power was kept below 10 $\mu$W. For the photocurrent (PC) measurements the devices were illuminated using a Fianium supercontinuum laser coupled to a monochromator,

providing a beam having 2 nm spectral width and stabilized power. The nominal laser power that we used for these measurements was typically 10 $\mu$W. The light exiting the monochromator was coupled onto the device using an optical microscope with long working distance objectives producing a spot of approximately 1 $\mu$m in diameter that could be focused anywhere on the device. All the measurements were done in a vacuum chamber with a window providing optical access to the device, which was mounted on a piezoelectric driven x-y stage, allowing positioning with a 50 nm precision.

# S2 FET output curves for $WSe_2/MoSe_2$ interface

In Figure 3a of the main text we have shown the output curves of a transistor realized on a $WSe_2/MoS_2$ interface, exhibiting the expected behavior (linear, saturation, and ambipolar injection regimes). For completeness, here we show (see Figure S1) the same transistor curves measured on a device realized on a $WSe_2/MoSe_2$ interface, which again exhibits the expected FET behavior. Specifically, at low $V_{SD}$ (for $V_G$ = 1.15 V and 1.2 V) the source-drain current increases linearly until $V_{SD}$ value reaches $\simeq V_G$-$V_{th}^{e/h}$ above which $I_{SD}$ saturates and stays constant (*pinch-off*). At much larger $V_{SD}$ values, $I_{SD}$ starts increasing steeply, which is the behavior expected when entering the ambipolar injection regime (*i.e.,* the regime in which both types of charge carriers are simultaneously injected into the channel from opposite contacts).

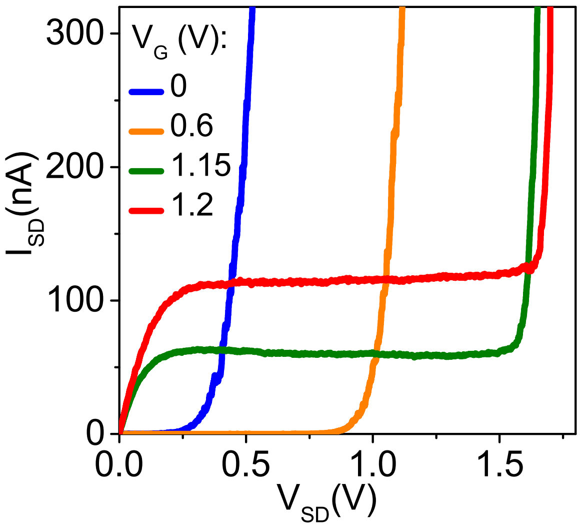


Figure S1. Source-drain current $I_{SD}$ as a function of source-drain bias $V_{SD}$ for different $V_G$ values (FET output curves) measured on a transistor realized on a $WSe_2/MoSe_2$ interface.

## S3 Photocurrent spectra of interfaces and their constituents

In the main text we have compared the photocurrent spectra measured on $WSe_2/MoSe_2$ and $WSe_2/MoS_2$ interfaces, to the photoluminescence spectra of the same interfaces. The goal there was to show that the onset of photocurrent occurs at an energy much smaller than the energy of all intralayer optical transitions, because in interfaces photocurrent is generated also through interlayer transitions. For completeness, in Figure S2 we show the comparison of the spectral dependence of the photocurrent measured on each interface with the photocurrent spectra of the constituent monolayers. The data confirm the conclusions drawn in the main text. For instance, Figure S2a shows that the onset of the photocurrent for the $WSe_2/MoSe_2$ interface (solid blue curve) clearly occurs at an energy much lower than that of the photocurrent of the constituent materials. In particular, at the energy of the interlayer exciton (shallow peak at 1.36 eV) present in the interface spectrum, no photosensitivity is observed in the spectra of the constituent layers (green and red lines correspond to $MoSe_2$ and $WSe_2$ monolayers respectively). The photocurrent of the interface increases steeply once the excitation

energy matches the single particle gap of the interface confirming the direct nature of the corresponding optical transition. Analogous data for the $WSe_2/MoS_2$ system are shown in Figure S2b. We see that photosensitivity is present at photon energies much lower than the gap of the constituent monolayers and that the photocurrent sets in at energies close to 1 eV, i.e., near the value of the single particle gap extracted from our transport measurement. Note how in all cases the photocurrent increase associated to a direct transition exhibits a steep onset (irrespective of whether the transitions are intralayer or interlayer). In contrast, the photocurrent increase starting at 1 eV that we see in Figure 2Sb for the $WSe_2/MoS_2$ interface is not steep, indicating the indirect nature of the optical transition in this case.

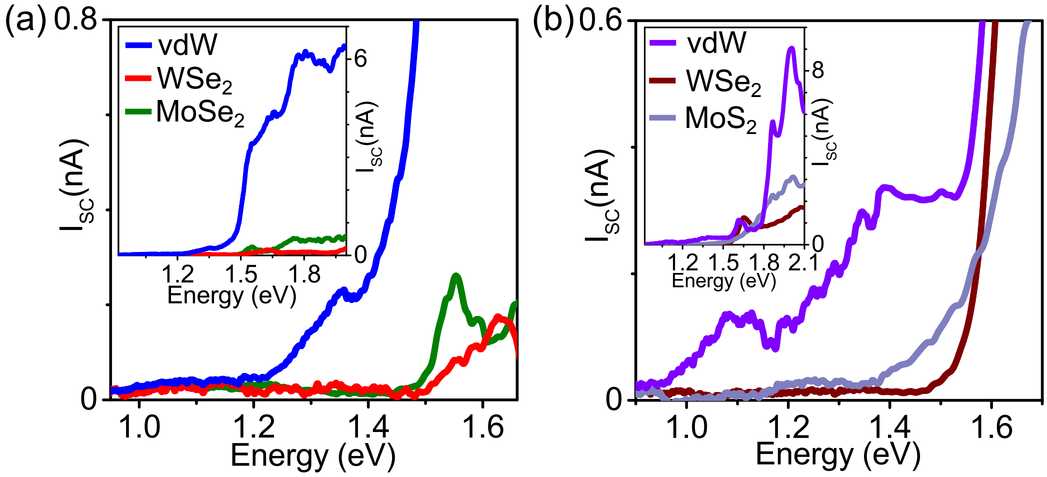


Figure S2. (a) Short-circuit current, $I_{SC}$, as function of incident photon energy for the $WSe_2/MoSe_2$ interface (blue line), and the $WSe_2$ (red line) and $MoSe_2$ (green line) individual monolayers. (Inset) Same data shown in panel (a) plotted for a larger range of excitation energies. (b) Short-circuit current, $I_{SC}$, as function of incident photon energy for $WSe_2/MoS_2$ interface (blue line), $WSe_2$ (brown line) and $MoS_2$ (grey line) individual monolayers. For both interfaces it is clear that the photocurrent measured on the interface starts at much lower energies than in the constituent monolayers.

## S4 Scanning photocurrent microscopy

In the main text we have discussed the spectral dependence of the photocurrent measured in our devices, and not the magnitude that – as we mentioned – depends on many

experimental details of the structure and of the conditions under which the measurements are done. To illustrate this last point, here we show a map of the short-circuit current $I_{\mathrm{SC}}$ (i.e., of the photocurrent) obtained by scanning the laser spot over the surface of a representative $WSe_2/MoS_2$ device (whose optical microscope image is shown in Figure S3b). The magnitude of the photocurrent depends on the position of the illumination spot and reverts its sign as the illumination spot is displaced from one contact to the other. That is the behavior expected in this measurement configuration, because the net photocurrent is determined from the imbalance of photoexcited carriers that exit the device at the two contacts (for a discussion see, for instance, Ref. 1). This map clearly shows that the magnitude of the photocurrent depends on the way the device is illuminated (it would also depend on many other parameters, such as, for instance, the gate voltage). The spectral dependence of $I_{\mathrm{SC}}$, however, is the same irrespective of these details, as we verified by measuring it at different positions of the illumination spot.

To exclude any possible effect of the contacts on $I_{SC}$ we also probe the photocurrent response of interface FETs in the presence of a p-n junction formed inside the channel away from the contacts. In ionic-liquid gated FET a lateral p-n junction can be defined and controlled electrostatically upon driving the transistor into the ambipolar injection regime (*i.e.,* the regime in which both types of charge carriers are simultaneously present in the FET channel, see Figure 3a (main text) for $V_G$ = 0.6 V) as has been demonstrated for multiple occasions.[2–4] Once the p-n junction is created and its position is defined by the appropriate bias conditions, the device is cooled down to T = 77 K, below the freezing point of the liquid, which immobilizes the ions in such a way that the p-n junction is also "frozen" in the transistor channel. Figure S3c shows the $I_{SD}$ vs $V_{SD}$ curve measured after cool down, with the rectifying behavior confirming the presence of the p-n junction. The presence of the p-n junction is also demonstrated by the photocurrent map (Figure S3d). Indeed the photocurrent is observed to peak in the center of the channel where the p-n junction is, and not anymore

at the contact (as shown in Figure S3b for the unbiased device). We have checked that the photocurrent spectra acquired from the p-n junction region coincide with the ones observed when the contacts are illuminated, indicating that the photocurrent probes the interface properties and is not influenced by contact effects.

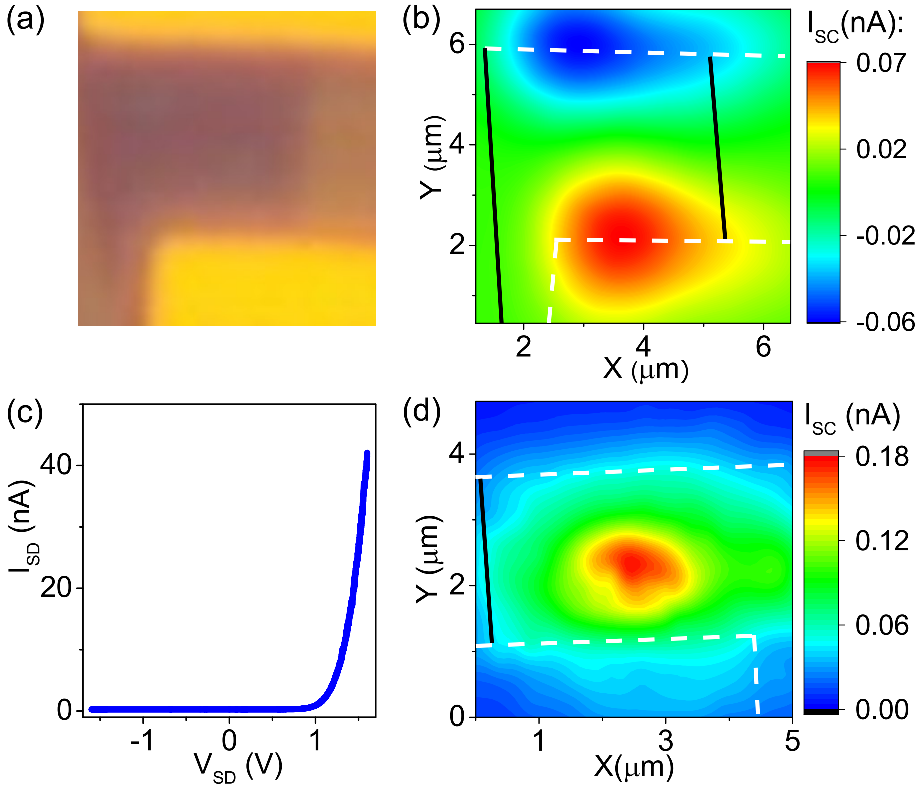


Figure S3. (a) Optical microscope image of the sample area from which the PC map shown in panel (b) was collected.(b) Photocurrent map (*i.e.*, $I_{SC}$ as a function of illumination position) measured on a $WSe_2$/$MoS_2$ interface transistor upon illumination with a 1125 nm (1.1 eV) excitation wavelength. The edges of the metal contacts and of the $WSe_2$/$MoS_2$ interface are indicated with the white dashed and solid black lines respectively. (c) Source-drain current $I_{SD}$ as a function of source-drain voltage $V_{SD}$ acquired after driving the FET into ambipolar injection regime at room temperature and cooling it down to T = 77K. Rectification of the $I_{\mathrm{SD}}$ indicates the formation of the p-n junction. (d) Photocurrent map measured on a $WSe_2$/$MoSe_2$ interface transistor in the presence of a p-n junction formed by cooling down the ionic liquid to T = 77K upon illumination with a 750 nm (1.65 eV) excitation wavelength.

# References


1. Ubrig, N.; Jo, S.; Berger, H.; Morpurgo, A. F.; Kuzmenko, A. B. Scanning Photocurrent Microscopy Reveals Electron-Hole Asymmetry in Ionic Liquid-Gated $WS_2$ Transistors. *Appl. Phys. Lett.* **2014**, *104*.

2. Zhang, Y. J.; Oka, T.; Suzuki, R.; Ye, J. T.; Iwasa, Y. Electrically Switchable Chiral Light-Emitting Transistor. *Science* **2014**, *344*, 725–729.

3. Jo, S.; Ubrig, N.; Berger, H.; Kuzmenko, A. B.; Morpurgo, A. F. Mono- and Bilayer $WS_2$ Light-Emitting Transistors. *Nano Letters* **2014**, *14*, 2019–2025.

4. Onga, M.; Zhang, Y.; Suzuki, R.; Iwasa, Y. High Circular Polarization in Electroluminescence from $MoSe_2$. *Appl. Phys. Lett.* **2016**, *108*, 2–6.
